# Supplementary material for: 3DPR: Single Image 3D Portrait Relight using Generative Priors
Source: arXiv:2510.15846 source file (2025-10-17)
Supplement: Supplementary file 10 [file output-figure18.pdf]

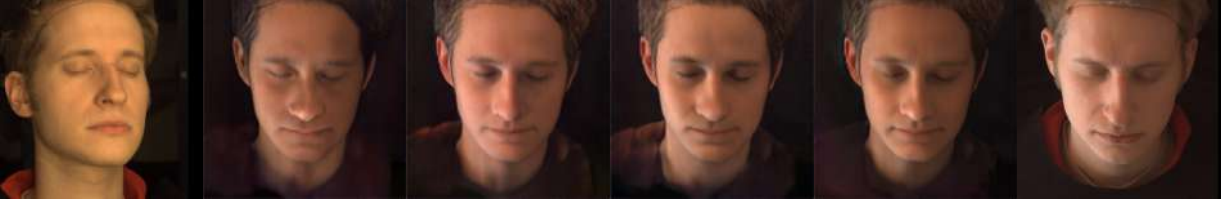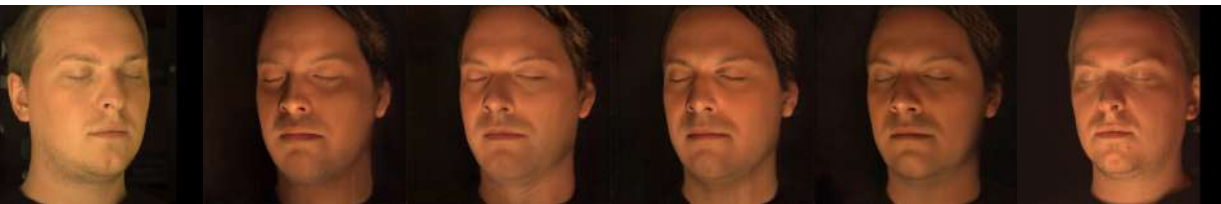

Input

$n = 5$

$n = 25$

$n = 100$

$n = 250$

GT

**Temporary page!**

$\LaTeX$  was unable to guess the total number of pages correctly. As there was some unprocessed data that should have been added to the final page this extra page has been added to receive it.

If you rerun the document (without altering it) this surplus page will go away, because  $\LaTeX$  now knows how many pages to expect for this document.
